# Supplementary material for: Measuring and Controlling Split Layer Privacy Leakage Using Fisher Information
Source: arXiv:2209.10119 source file (2022-09-21)
Supplement: Supplementary file 1 [file appendix.tex]

\begin{figure}
    \centering
    \begin{subfigure}{0.49\textwidth}
        \centering
        \includegraphics[width=\textwidth]{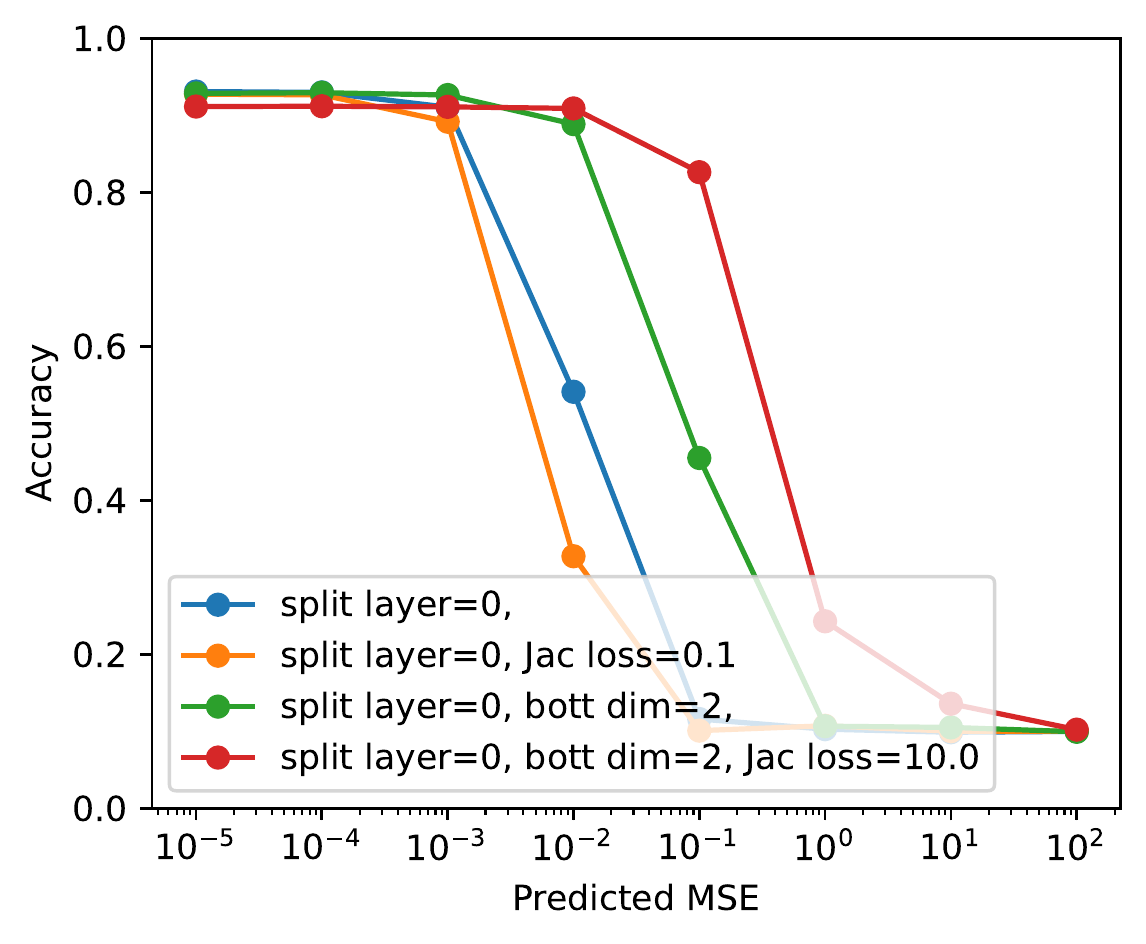}
        \caption{TODO}
        \label{fig:eval_resnet_split0}
    \end{subfigure}
    \begin{subfigure}{0.49\textwidth}
        \centering
        \includegraphics[width=\textwidth]{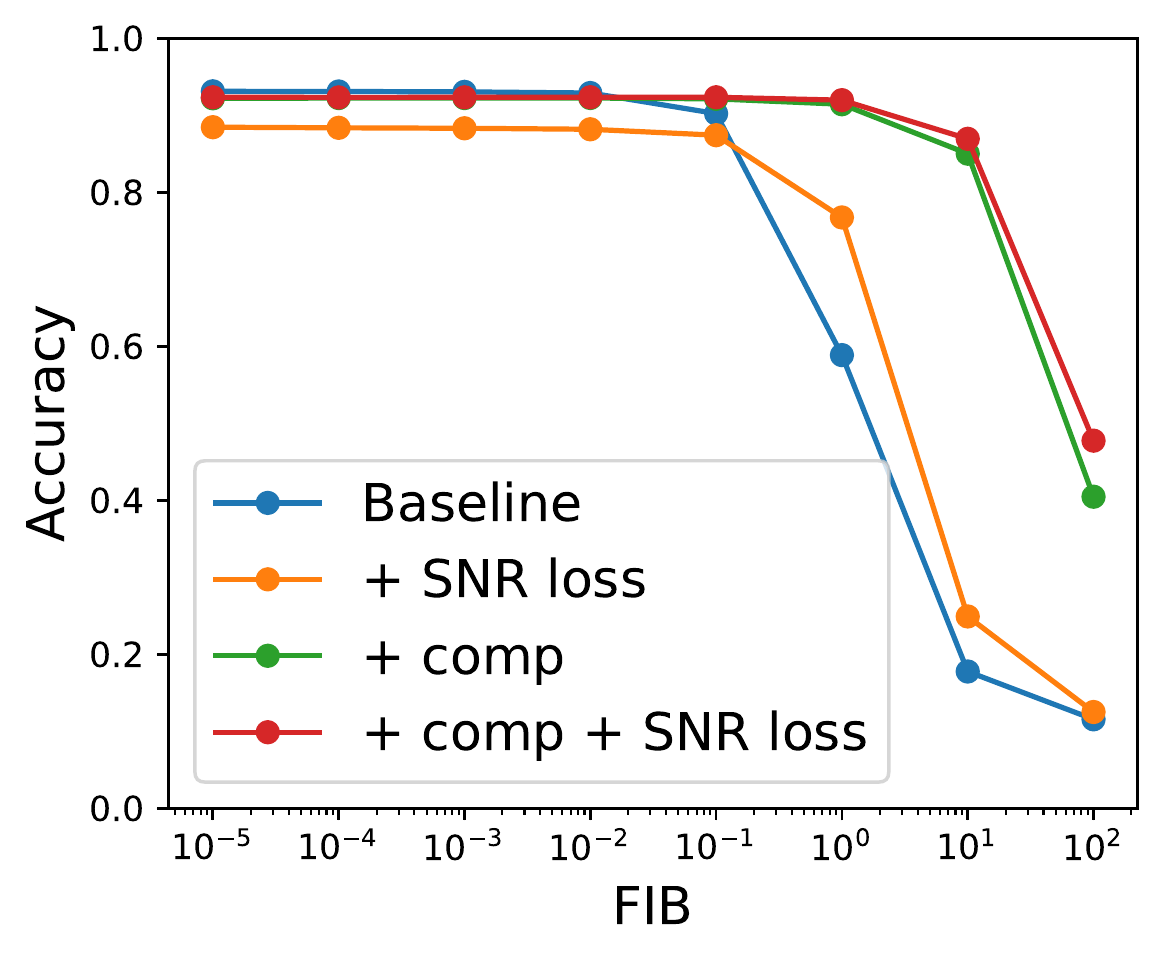}
        \caption{Image model, split-middle}
        \label{fig:eval_resnet_split7}
    \end{subfigure}
    \begin{subfigure}{0.49\textwidth}
        \centering
        \includegraphics[width=\textwidth]{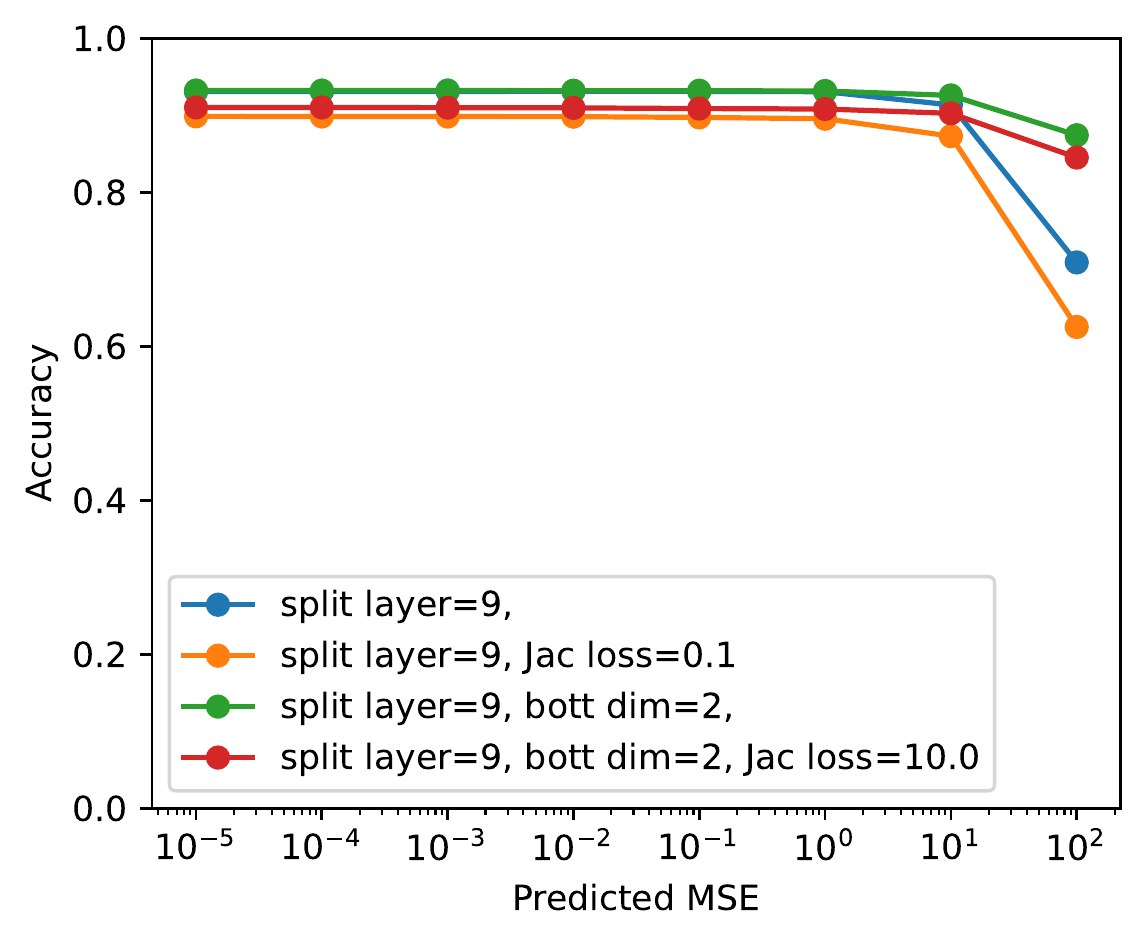}
        \caption{TODO}
        \label{fig:eval_resnet_split9}
    \end{subfigure}
    \begin{subfigure}{0.49\textwidth}
        \centering
        \includegraphics[width=\textwidth]{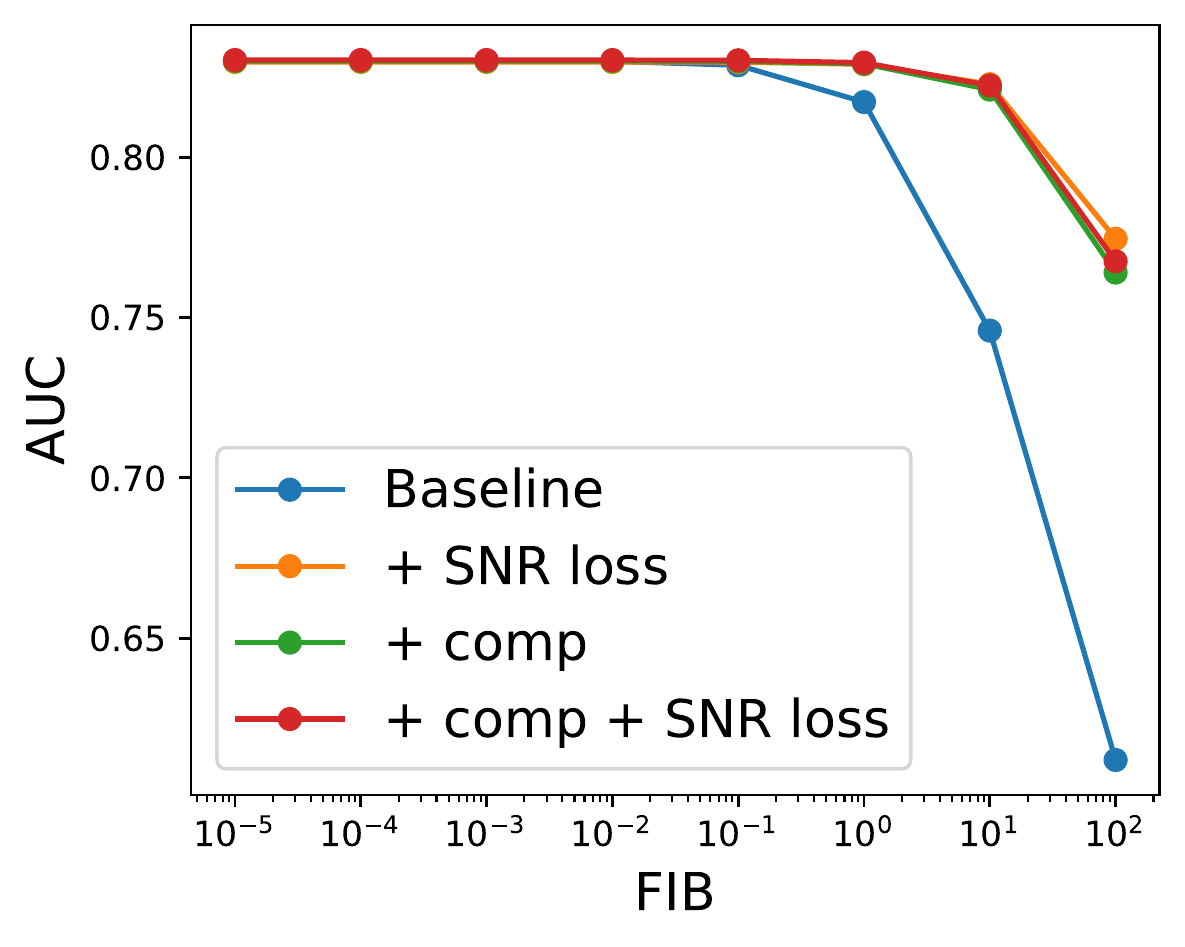}
        \caption{Recommendation model}
        \label{fig:eval_movielens_split0}
    \end{subfigure}
    \caption{Introducing compression/decompression layers (comp) or SNR loss improves the privacy-utility trade-off. \textcolor{red}{TODO: Baseline > No opt & put horizontal "original accuracy line"}}
    \label{fig:eval_accuracy_utility}
\end{figure}
